# Supplementary material for: Theory of electron-plasmon coupling in semiconductors
Source: arXiv:1609.02843 source file (2016-09-09)
Supplement: Supplementary file 1 [file supplemental.pdf]

# Supplemental Material for
# "Theory of electron-plasmon coupling in semiconductors"

Fabio Caruso and Feliciano Giustino
*Department of Materials, University of Oxford, Parks Road, Oxford, OX1 3PH*

## CONVERGENCE OF THE PLASMON-INDUCED BAND GAP RENORMALIZATION

In Fig. S1(a–c) we illustrate the convergence of the energy-level renormalization of silicon as a function of the broadening parameter $\eta$. Figure S1(d–f) show the convergence with respect to the number of bands included in the summation over states in the construction of the electron-plasmon self-energy. Based on these tests we employed 10 bands in all calculations (4 valence bands and 6 conduction bands). The relatively fast convergence with respect to unoccupied states was to be expected, because the characteristic energy scale in the electron-plasmon self-energy is the energy of thermal plasmons. In the related case of $GW$ calculations the characteristic energy scale is that of bulk plasmons, hence considerably larger energy cutoffs are typically necessary. We also note that the electron-plasmon matrix elements near $\mathbf{q} = 0$ provide the main contribution to the Brillouin-zone integration. Since for $\mathbf{q} \to 0$ we have $M^{mn}(\mathbf{k}, \mathbf{q}) \simeq \delta_{mn}$, with $\delta_{mn}$ the Kronecker delta, the summation over bands in the electron-plasmon self-energy is dominated by the $n = m$ term. In order to test the convergence with respect to Brillouin-zone sampling we considered grids with $30^3$ and $40^3$ points and a carrier concentration of $2.5 \cdot 10^{20}$ cm$^{-3}$. For these two cases we obtained $\Delta E_c = -37/38$ meV, $\Delta E_v = 30/31$ meV, and $\Delta E_{\rm g} = -68/69$ meV. These values confirm that our choice of using $40^3$ points in all calculations yields fully converged results.

To estimate the effect of temperature on the electron-plasmon interactions, we calculated the BGN as a function of temperature up to 1000 K for carrier concentrations of $2.5 \cdot 10^{19}$ cm$^{-3}$ and $2.5 \cdot 10^{20}$ cm$^{-3}$. In our calculations, temperature is included for both electrons and plasmons via the Fermi/Bose distribution in Eq. (1) and is illustrated in Fig. S2, where we report the difference $\mathrm{BGN}(T) - \mathrm{BGN}(T = 0)$. These calculations reveal that the BGN changes by less than 1 meV for temperatures up to 600 K. The weak temperature dependence stems from the relatively large ratio between the plasmon energy and the thermal energy at room temperature $\hbar\omega_{\rm P}/k_B T \simeq 4 - 6$, which makes the thermal excitation of plasmons unlikely.

## COMPUTATIONAL PARAMETERS FOR THE GROUND-STATE CALCULATIONS

Ground-state calculations were performed within the local density approximation (LDA) to density functional theory [1, 2], (DFT) as implemented in the `Quantum ESPRESSO` distribution [3]. We used norm-conserving Troullier-Martins pseudo-potentials [4], a 40 Ry planewaves kinetic energy cutoff, and sampled the Brillouin zone with a 10×10×10 Monkhorst-Pack grid. Doped silicon was described using the 'rigid-band model', that is by rigidly shifting the Fermi energy into the conduction band and keeping the electron density of the undoped system. As a sanity check, in the case of $n = 2 \cdot 10^{20}$ cm$^{-3}$ we repeated these calculations within the 'jellium model', that is by explicitly including extra electrons in the unit cell and adding a uniform positive compensating background. The results were essentially identical to those of the rigid-band calculation.

## COMPUTATION OF THE SCATTERING RATES AND RELAXATION TIMES

All scattering rates $\Gamma_{n\mathbf{k}}$ and relaxation times $\tau_{n\mathbf{k}}$ reported in this work have been obtained directly through the evaluation of the expressions:

$$\Gamma_{n\mathbf{k}} = 2\,\mathrm{Im}\,\Sigma_{n\mathbf{k}}/\hbar, \tag{S1}$$

$$\tau_{n\mathbf{k}} = \hbar/2\,\mathrm{Im}\,\Sigma_{n\mathbf{k}}, \tag{S2}$$

where $\Sigma_{n\mathbf{k}}$ is the self-energy for each interaction. We computed Eqs. (S1-S2) by accounting explicitly for the interaction of electrons with plasmons, phonons, electron-hole pairs, and impurities. This has been achieved through the evaluation of the electron-plasmon self-energy ($\Sigma^{\rm eP}_{n\mathbf{k}}$), the electron-phonon self-energy ($\Sigma^{\rm ep}_{n\mathbf{k}}$), the contribution of electron-hole pairs ($\Sigma^{\rm eh}_{n\mathbf{k}}$), and the impurity self-energy ($\Sigma^{\rm i}_{n\mathbf{k}}$). The total relaxation time has thus been obtained from Matthiessen's rule $\tau^{\rm tot}_{n\mathbf{k}} = \hbar/2\,\mathrm{Im}(\Sigma^{\rm ep}_{n\mathbf{k}} + \Sigma^{\rm eP}_{n\mathbf{k}} + \Sigma^{\rm eh}_{n\mathbf{k}} + \Sigma^{\rm i}_{n\mathbf{k}})$. In the following, we provide the details for the computation of the self-energy for each of these scattering mechanisms.

### Scattering rates and relaxation times due to plasmons

For numerical calculations of the electron-plasmon self-energy it is convenient to avoid the computation of the

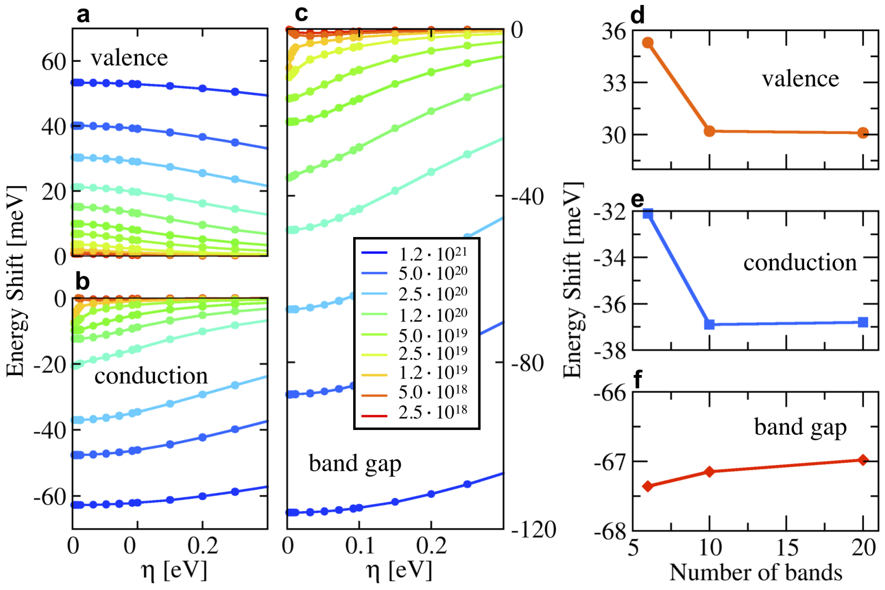


Figure S1. (a) Energy-level renormalization from the electron-plasmon interaction, calculated using Eq. (1) for the valence band top of silicon, $\Delta E_v$. We show the convergence of the energy shift with respect to the broadening parameter $\eta$, for several values of the carrier density (each curve is for one carrier density). (b) Same as in (a), but for the conduction band bottom of silicon, $\Delta E_c$. (c) Band gap renormalization, $\Delta E_{\rm g} = \Delta E_c - \Delta E_v$, as obtained from the curves in (a) and (b). Based on these convergence tests we set the broadening parameter to $\eta$ = 10 meV in all the calculations discussed in the main text. (d–f) Convergence of the energy-level renormalization by electron-plasmon interaction as a function of the number of bands $m$ included in Eq. (1): we report the convergence of $\Delta E_v$, $\Delta E_c$, and $\Delta E_{\rm g}$ in (d), (e), and (f), respectively.

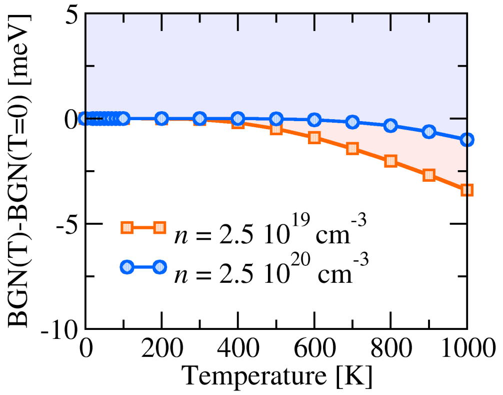


Figure S2. Temperature dependence of the BGN for carrier concentrations of $2.5 \cdot 10^{19}$ cm$^{-3}$ and $2.5 \cdot 10^{20}$ cm$^{-3}$.

partial derivative of the dielectric matrix with respect to frequency. Following Ref. [5], we determined the changes of the dielectric matrix induced by doping from:

$$\Delta\epsilon^{-1}(\mathbf{q},\omega) = \epsilon^{-1}_{\mathbf{G}=0,\mathbf{G}'=0}(\mathbf{q},\omega)\big|_{\rm D} - \epsilon^{-1}_{\mathbf{G}=0,\mathbf{G}'=0}(\mathbf{q},\omega)\big|_{\rm I}, \tag{S3}$$

where D and I stand for 'doped' and 'insulator', respectively. Since electron-hole transitions are not allowed for momenta below the critical cutoff $q_c$, $\Delta\epsilon^{-1}$ coincides with the contribution of thermal plasmons, that is, $\Delta\epsilon^{-1}(\mathbf{q},\omega) = \left[\frac{\partial\epsilon(\mathbf{q},\omega)}{\partial\omega}\right]^{-1}_{\omega_{\rm P}(\mathbf{q})} \frac{2\,\omega_{\rm P}(\mathbf{q})}{\omega^2-\omega^2_{\rm P}(\mathbf{q})}$. These quantities may be combined to obtain:

$$\left[\frac{\partial\epsilon(\mathbf{q},\omega)}{\partial\omega}\right]^{-1}_{\omega_{\rm P}(\mathbf{q})} = -\frac{1}{2}\omega_{\rm P}(\mathbf{q}) \left[\epsilon^{-1}_{\mathbf{G}=0,\mathbf{G}'=0}(\mathbf{q},\omega=0)\big|_{\rm D} - \epsilon^{-1}_{\mathbf{G}=0,\mathbf{G}'=0}(\mathbf{q},\omega=0)\big|_{\rm I}\right]. \tag{S4}$$

Our numerical strategy for the computation of the electron-plasmon self-energy combines Eqs. (1), (2), and (S4).

In practice, for each doping level we perform two separate calculations of inverse dielectric matrices using the random-phase approximations to obtain $\epsilon^{-1}_{\mathbf{G}=0,\mathbf{G}'=0}(\mathbf{q},\omega = 0)\big|_{\rm I/D}$. The electron-plasmon coupling coefficients are computed using optical matrix elements from `Yambo` [6]. The single-particles eigenvalues $\epsilon_{n\mathbf{k}}$ and eigenstates $\psi_{n\mathbf{k}}$ have obtained from DFT, employing the computational parameters listed above, in the section "Ground-state calculation". We determined the plasmon frequency $\omega_{\rm P}$ at each wavevector $\mathbf{q}$ through first principles calculations of the loss functions in the random-phase approximation, as implemented in `Yambo`. In particular, the loss function has been computed for each doping concentration, and for each momentum in the Brillouin zone, on a homogeneous Monkhorst-Pack grid consisting of 40×40×40 k-points. These calculations are exemplified in Fig. S3 (a), where we report the

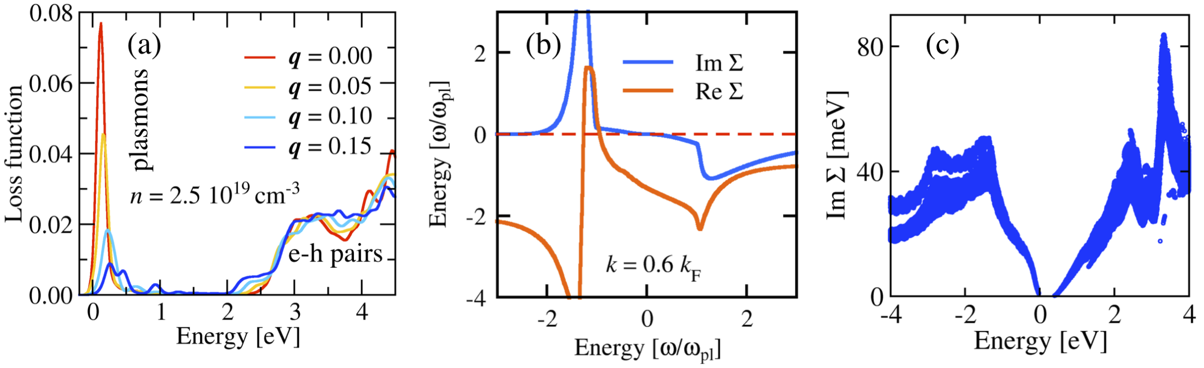


Figure S3. (a) Loss function of silicon for several momenta (in units of $2\pi/a$, with $a$ being the lattice constant of silicon) along the Γ-X high-symmetry line. The thermal plasmons correspond to the sharp peaks on the left, whereas higher energy features are related to electron-hole transitions. (b) Real and imaginary part of the *GW* self-energy of the homogeneous electron gas in units of the plasmon energy ($\omega_{\rm pl}$) for a Wigner-Seitz radius $r_s = 5$, effective mass $m_{\rm eff} = 1$, and momentum $k = 0.6\,k_{\rm F}$. (c) Imaginary part of the electron self-energy due to electron-phonon interaction.

loss function of silicon at Γ for a doping concentration of $10^{19}$ cm$^{-3}$. The signatures of thermal plasmons and electron-hole pairs are indicated. The loss-function *maps* reported in Fig. 1 (a-c) have been obtained by combining several loss-function calculations for finite momentum transfers along the Γ-X high-symmetry line in the first Brillouin zone.

## Scattering rates and relaxation times due to electron-hole pairs

As discussed in the main text of the manuscript, *inter*band electron-hole excitations must have energies larger than the fundamental gap, and do not contribute to the scattering of low-energy carriers. Correspondingly, only in the vicinity of the Fermi energy low-energy *intra*band transitions are allowed. To accounts for these effects, we approximate the extrinsic carriers as an homogeneous electron gas (HEG) with band dispersion given by $\epsilon_{\mathbf{k}} = \hbar^2\mathbf{k}^2/2m_{\rm eff}$, where $m_{\rm eff}$ is the isotropic effective mass of silicon. The HEG approximation is well justified since the Fermi energy in all cases considered is extremely small (< 120 meV), and the energy vs. momentum dispersion relations are accurately described by a parabolic approximation.

In the *GW* approximation, Σ may be expressed as:

$$\Sigma(\mathbf{k},\omega) = \frac{i}{2\pi}\int d\omega' d\mathbf{q} G(\mathbf{k}+\mathbf{q},\omega+\omega')W(\mathbf{q},\omega')e^{i\delta\omega'}. \qquad \text{(S5)}$$

where $W$ is screened Coulomb interaction, defined by: $W(\mathbf{q},\omega) = v(\mathbf{q})\epsilon^{-1}(\mathbf{q},\omega)$. Here, $v(\mathbf{q}) = 4\pi e^2/\varepsilon_0 q^2$ is the bare Coulomb interaction and the dielectric function is given by $\epsilon(\mathbf{q},\omega) = 1 - v(\mathbf{q})\chi_0(\mathbf{q},\omega)$. $\chi_0$ is the irreducible polarizability which, for the homogeneous electron gas, may be computed analytically through the Lindhard formula (see, e.g., Ref. [7]). The scattering rates determined from Eq. (S5) account exclusively for the contribution of electron-hole pairs, since Im $\epsilon^{-1}(\mathbf{q},\omega)$ (and thus Im Σ) is zero at the plasmon energy [7].

We implemented the *GW* self-energy [Eq. (S5)] following Eqs. (56) and (90) of Ref. [8]. To validate our implementation, we report in Fig. S3 (b) the self-energy for an HEG density given by the Wigner-Seitz radius $r_s = 5$, and $m_{\rm eff} = 1$. These calculation are in excellent agreement with previously published data by Lundqvist [9]. The small differences arise from the use of the plasmon-pole approximation in Ref. [9], whereas in our work the full frequency dependence of the Lindhard function has been considered. The scattering rates and relaxation times have been obtained from Eqs. (S1-S2), and Eq. (S5) by taking the HEG density equal to the extrinsic carrier density.

## Scattering rates and relaxation times due to impurities

The scattering rates by impurities were calculated by considering a homogeneous electron gas (as in the previous section) in the presence of Coulomb scatterers randomly distributed, following the theory of Ref. [10]. More specifically, we evaluated the relaxation time $\tau^{\rm i}_{n\mathbf{k}}$ using:

$$\frac{1}{\tau^{\rm i}_{n\mathbf{k}}} = \frac{2\pi N_{\rm d} m_{\rm e} m^*}{\hbar^3}\int\frac{d\mathbf{k}'}{(2\pi)^3}\frac{\delta(k'-k_{\rm F})}{k'}\times \times\left|\frac{4\pi e^2/\epsilon_0}{\left[2k_{\rm F}\sin\left(\frac{\theta}{2}\right)\right]^2 + q^2_{\rm TF}}\right|^2, \qquad \text{(S6)}$$

where $N_{\rm d}$ is the dopant concentration, which we set equal to the carrier density; and $\theta$ denotes the angle between $\mathbf{k}$

and $\mathbf{k}'$; the isotropic effective mass is obtained as $m^* = 3/(2/m^*_\perp + 1/m^*_\parallel)$, where $m^*_\perp = 0.19$ and $m^*_\parallel = 0.89$ are the transverse and longitudinal effective masses. In practice, we consider an homogeneous electron gas with density equal to the dopant concentration $N_\mathrm{d}$. The Fermi momentum $k_\mathrm{F}$ is thus determined via $k_\mathrm{F} = (3\pi^2 N_\mathrm{d})^{\frac{1}{3}}$, whereas the Thomas-Fermi wavevector $q_\mathrm{TF}$ is given by $k_\mathrm{F} = (6\pi N_\mathrm{d}/\epsilon_\mathrm{F})^{\frac{1}{2}}$, with $\epsilon_\mathrm{F} = \hbar k_\mathrm{F}^2/2mm^*$ being the Fermi energy.

**Scattering rates and relaxation times due to phonons**

We estimate the effects of phonons to the electronic scattering rate and relaxation time from first principles through the evaluation of the electron-phonon self-energy:

$$\Sigma_{n\mathbf{k}} = \sum_{\nu m} \int \frac{d\mathbf{q}}{\Omega_\mathrm{BZ}} |g_{mn,\nu}(\mathbf{k},\mathbf{q})|^2 \left[ \frac{n(\omega_{\mathbf{q},\nu}) + f(\epsilon_{m,\mathbf{k+q}})}{\epsilon_{n,\mathbf{k}} - \epsilon_{m,\mathbf{k+q}} + \omega_{\mathbf{q},\nu} - i\eta} + \frac{n(\omega_{\mathbf{q},\nu}) + 1 - f(\epsilon_{m,\mathbf{k+q}})}{\epsilon_{n,\mathbf{k}} - \epsilon_{m,\mathbf{k+q}} - \omega_{\mathbf{q},\nu} - i\eta} \right], \tag{S7}$$

where the electron-phonon coupling coefficients are defined by

$$g_{mn,\nu}(\mathbf{k},\mathbf{q}) = \left( \frac{\hbar}{2m_0\omega_{\mathbf{q}\nu}} \right)^{1/2} \langle \psi_{m\mathbf{k+q}} | \partial_{\mathbf{q}\nu} V | \psi_{n\mathbf{k}} \rangle. \tag{S8}$$

Here $\partial_{\mathbf{q}\nu} V$ is the derivative of the self-consistent potential associated with a phonon of wavevector $\mathbf{q}$, branch index $\nu$, and frequency $\omega_{\mathbf{q}\nu}$. $n/f$ are Bose/Fermi occupation factors for phonons/electrons, respectively. Equation (S7) has been evaluated computed in the limit zero doping.

The calculations of electron-phonon coupling self-energy defined in Eq. S7 were performed using the `EPW` code [11, 12]. The DFT/LDA eigenvalues $\epsilon_{n,\mathbf{k}}$ and eigenvectors $\psi_{n\mathbf{k}}$ were computed by means of `Quantum ESPRESSO` [3] on a coarse 12×12×12 k-point grid. We thus computed the phonon frequencies $\omega_{\nu\mathbf{q}}$ and electron-phonon matrix elements $g_{mn,\nu}(\mathbf{k},\mathbf{q})$ using density functional perturbation theory [13] on a coarse 6×6×6 grid. All these quantities were subsequently Wannier-interpolated [14] on fine 40×40×40 meshes. We thus proceeded to the evaluation of the imaginary part of the electron-phonon self-energy, and the corresponding electron-phonon scattering rates, in the Migdal approximation following Ref. [11].

[1] P. Hohenberg and W. Kohn, Phys. Rev. **136**, B864 (1964).
[2] W. Kohn and L. J. Sham, Phys. Rev. **140**, A1133 (1965).
[3] P. Giannozzi *et al.*, J. Phys.: Condens. Matter **21**, 395502 (2009).
[4] N. Troullier and J. L. Martins, Phys. Rev. B **43**, 1993 (1991).
[5] Y. Liang and L. Yang, Phys. Rev. Lett. **114**, 063001 (2015).
[6] A. Marini, C. Hogan, M. Grning, and D. Varsano, Comp. Phys. Commun. **180**, 1392 (2009).
[7] G. Mahan, *Many-Particle Physics* (Springer, 2000).
[8] L. Hedin, Phys. Rev. **139**, A796 (1965).
[9] B. I. Lundqvist, Phys. Kondens. Mater. **7**, 117.
[10] S. Das Sarma and F. Stern, Phys. Rev. B **32**, 8442 (1985).
[11] J. Noffsinger, F. Giustino, B. D. Malone, C.-H. Park, S. G. Louie, and M. L. Cohen, Comp. Phys. Commun. **181**, 2140 (2010).
[12] F. Giustino, M. L. Cohen, and S. G. Louie, Phys. Rev. B **76**, 165108 (2007).
[13] S. Baroni, S. de Gironcoli, A. Dal Corso, and P. Giannozzi, Rev. Mod. Phys. **73**, 515 (2001).
[14] A. A. Mostofi, J. R. Yates, Y.-S. Lee, I. Souza, D. Vanderbilt, and N. Marzari, Comp. Phys. Commun. **178**, 685 (2008).
